# Supplementary material for: SVGDreamer: Text Guided SVG Generation with Diffusion Model
Source: arXiv:2312.16476 source file (2026-04-20)
Supplement: Supplementary file 1 [file supp_icon.pdf]

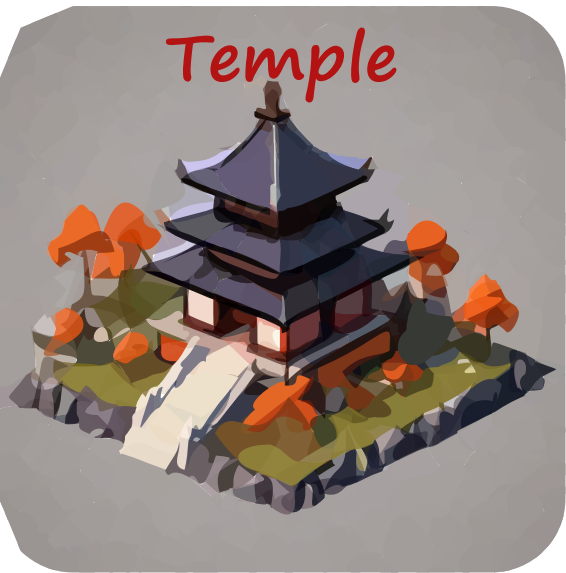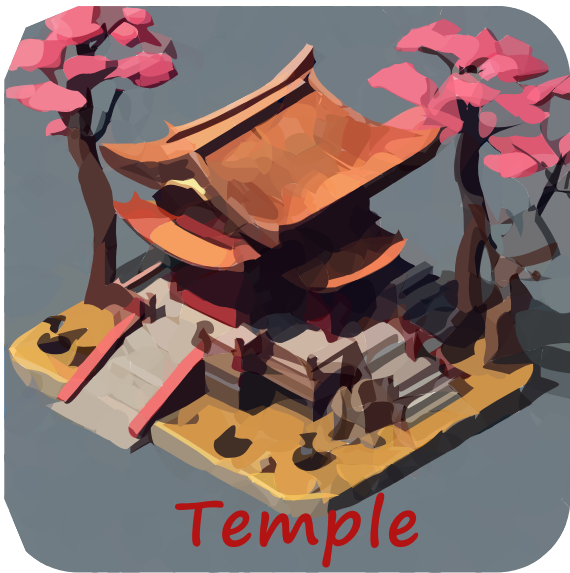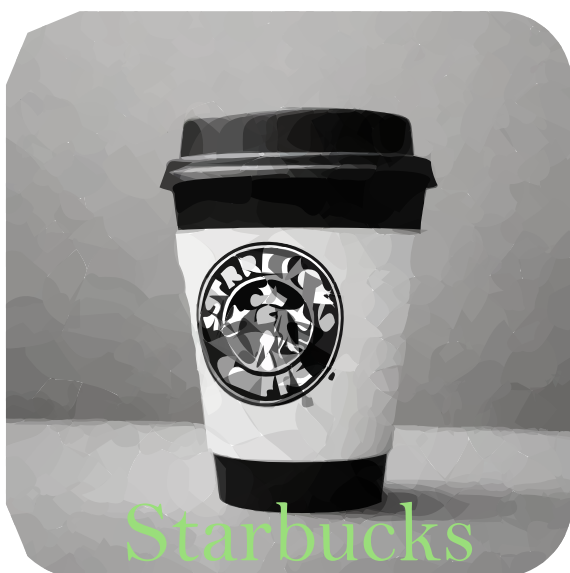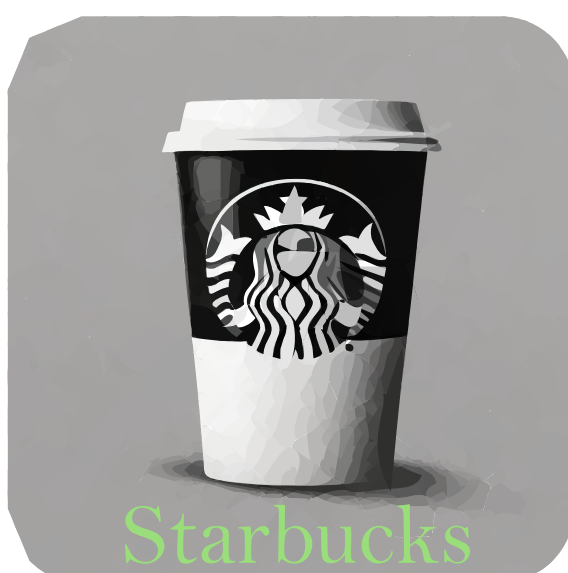

“The logo of the Japanese mystery temple,, game art, cartoon, 3d animation style”

“A Starbucks coffee cup in black and white”

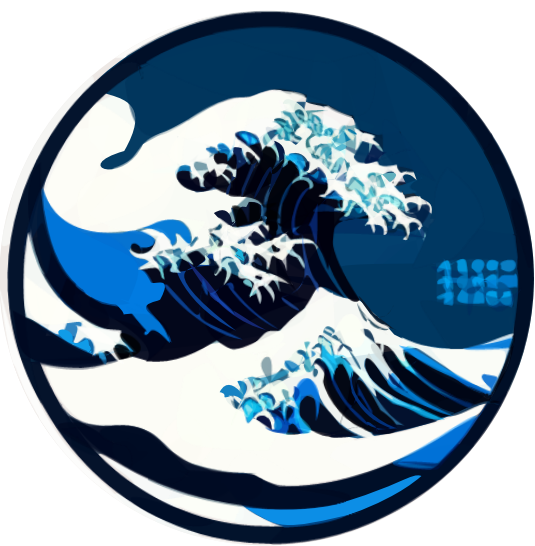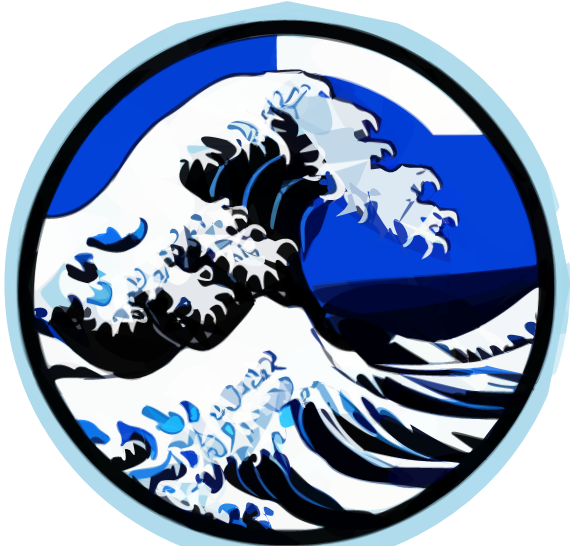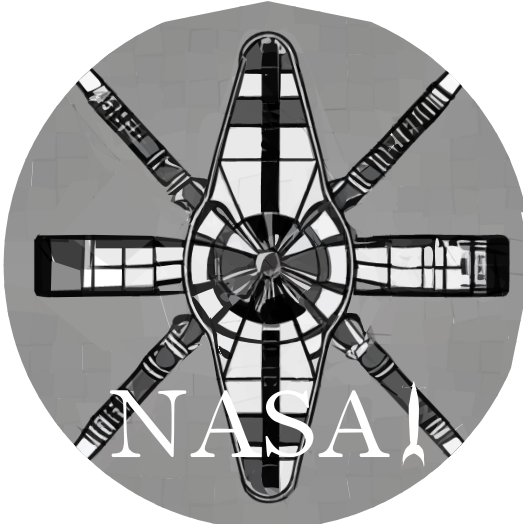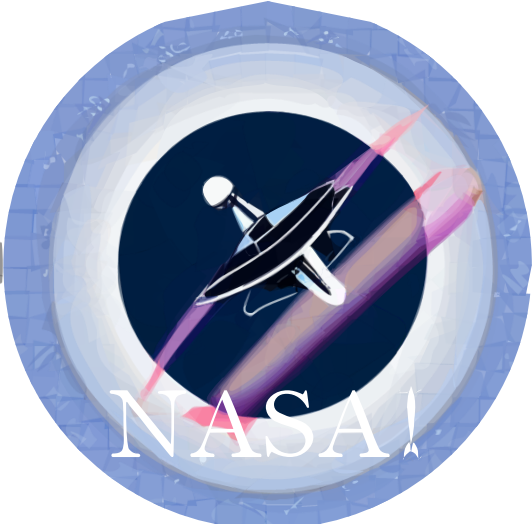

”Bold logo icon in blue, black, white colors for a simplified version of Great Wave of Kanagawa”

“An astronaut, the logo, vector art.”



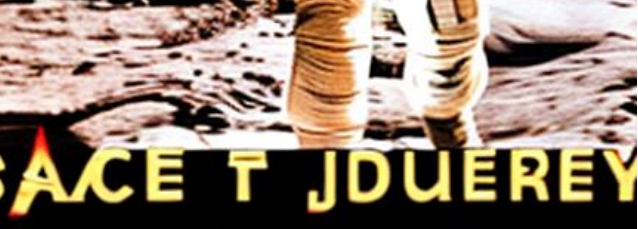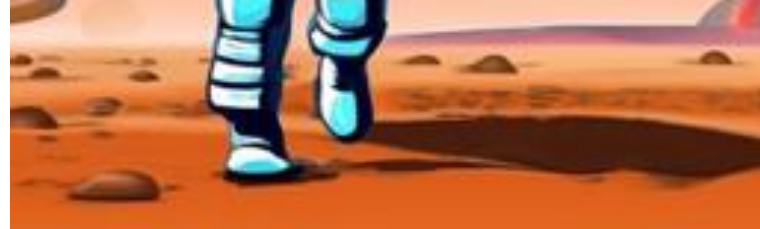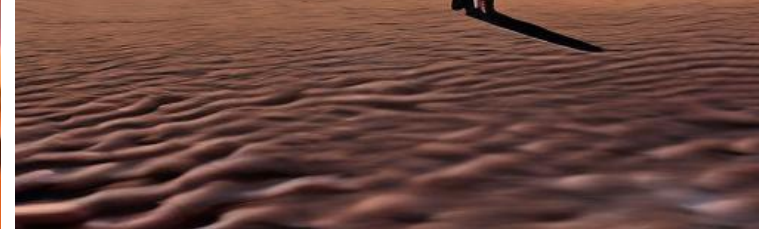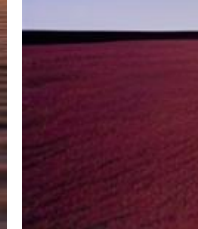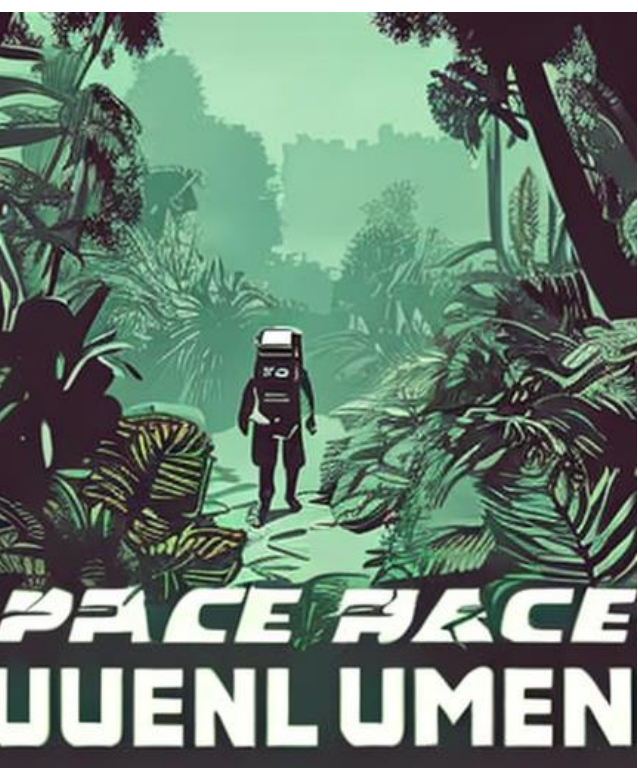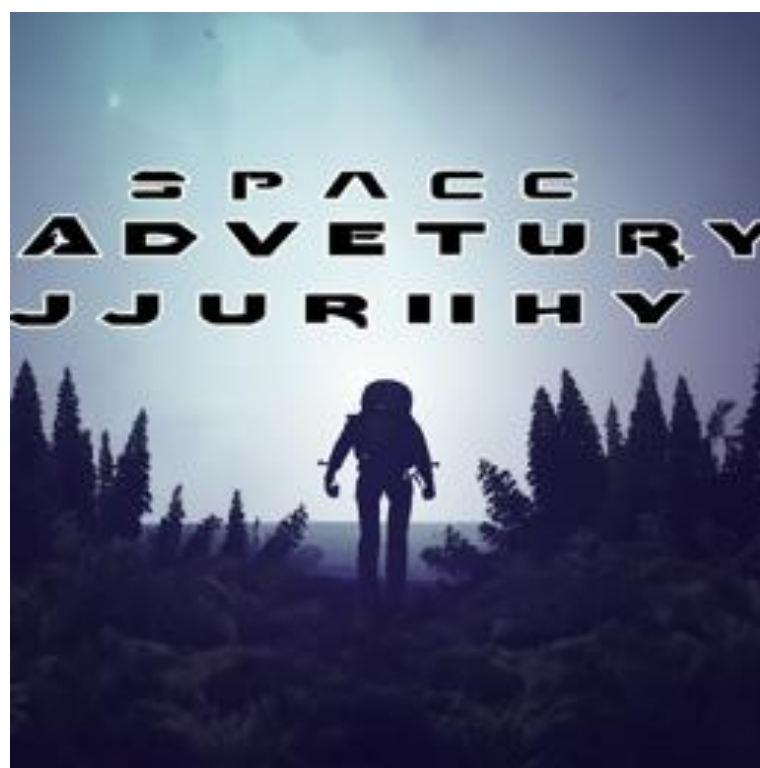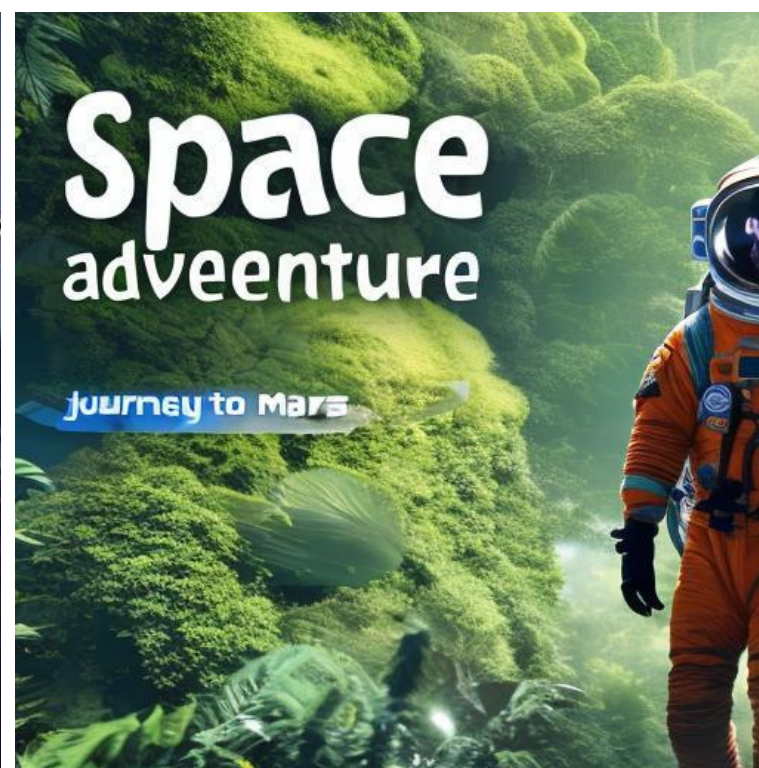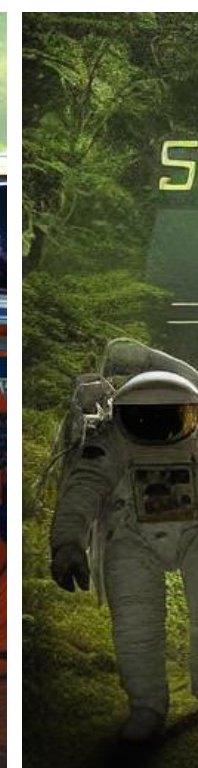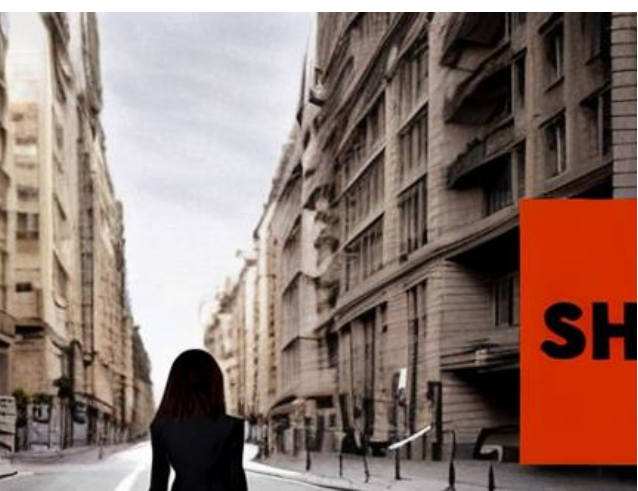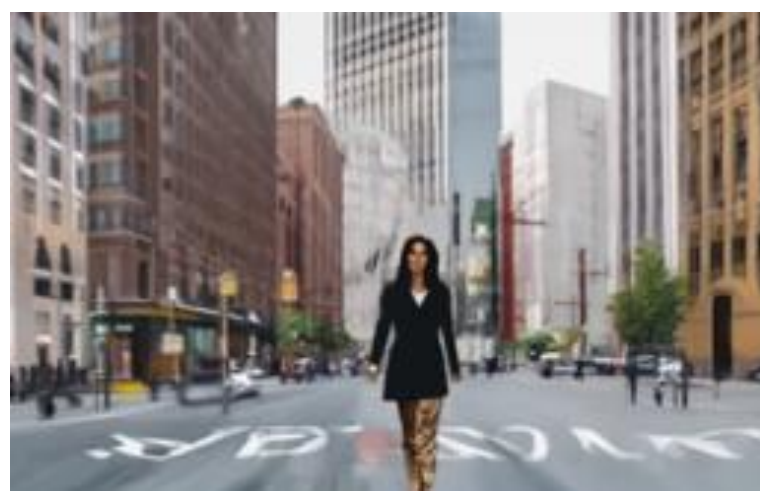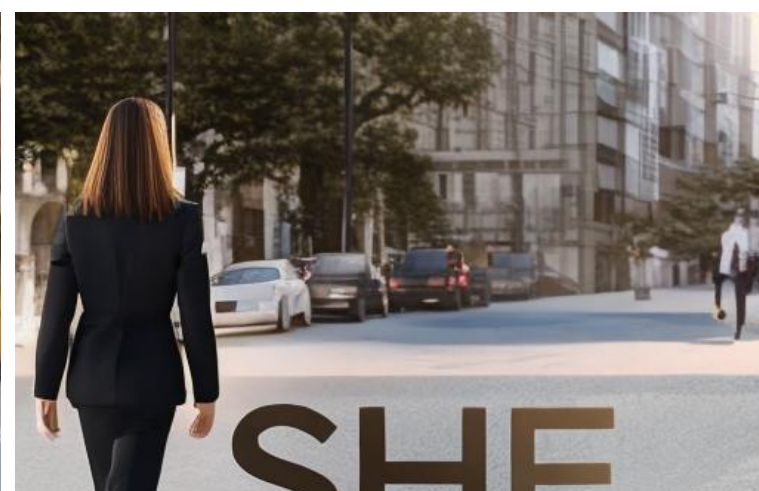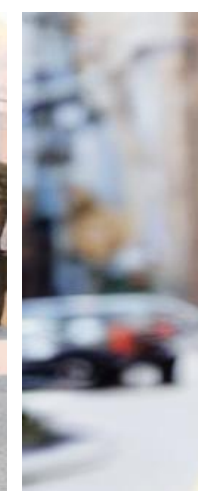



Seed 1

S

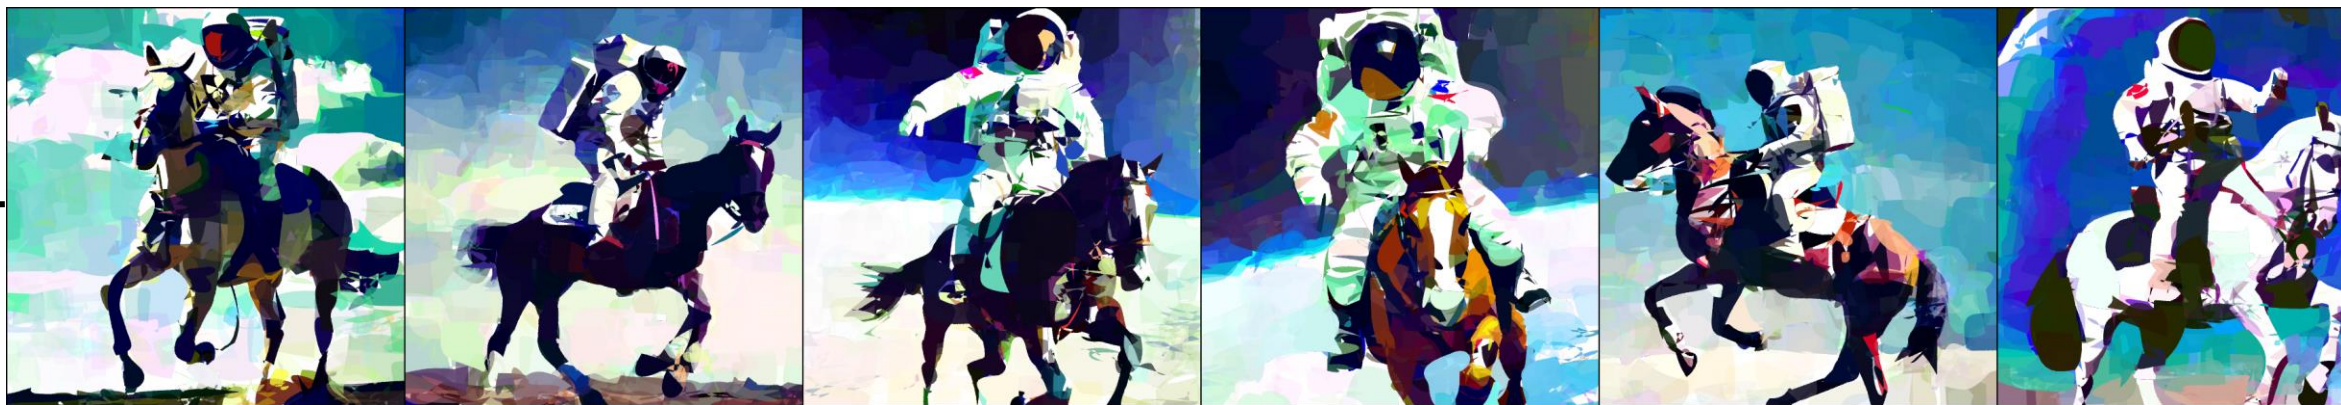

Seed 1

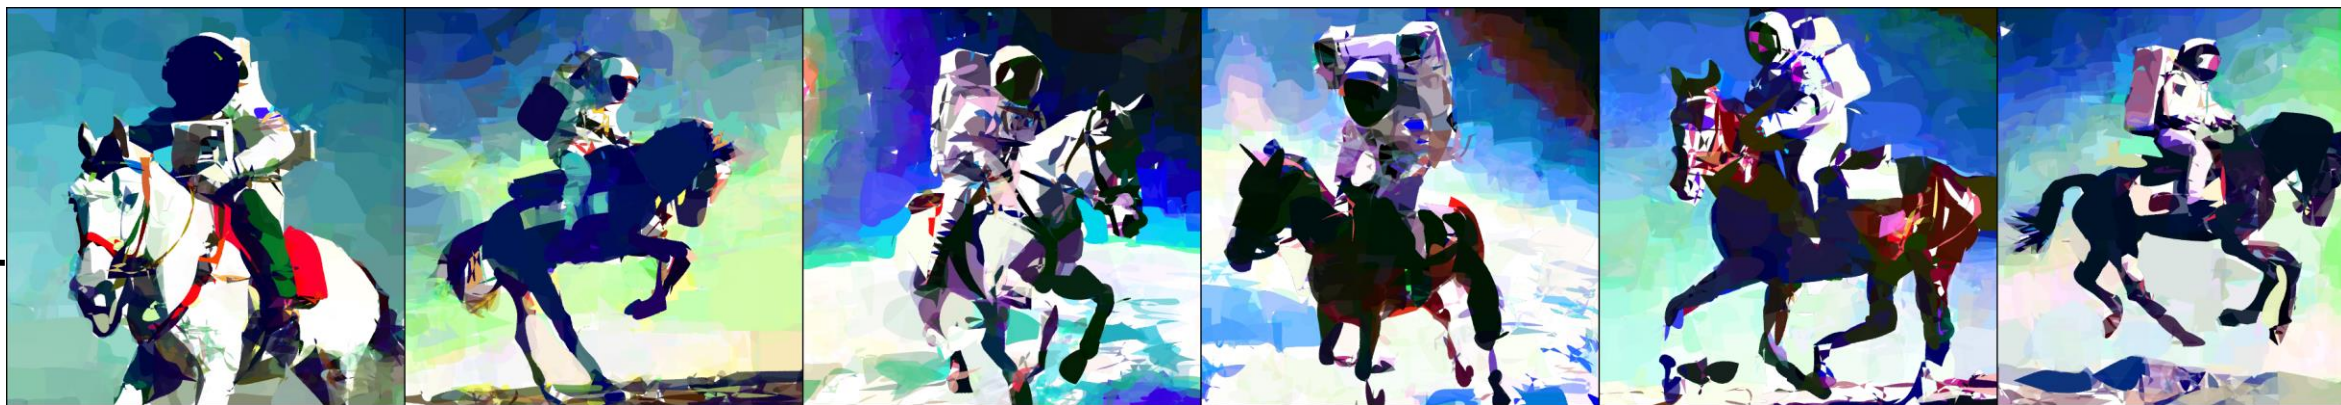

Seed 2

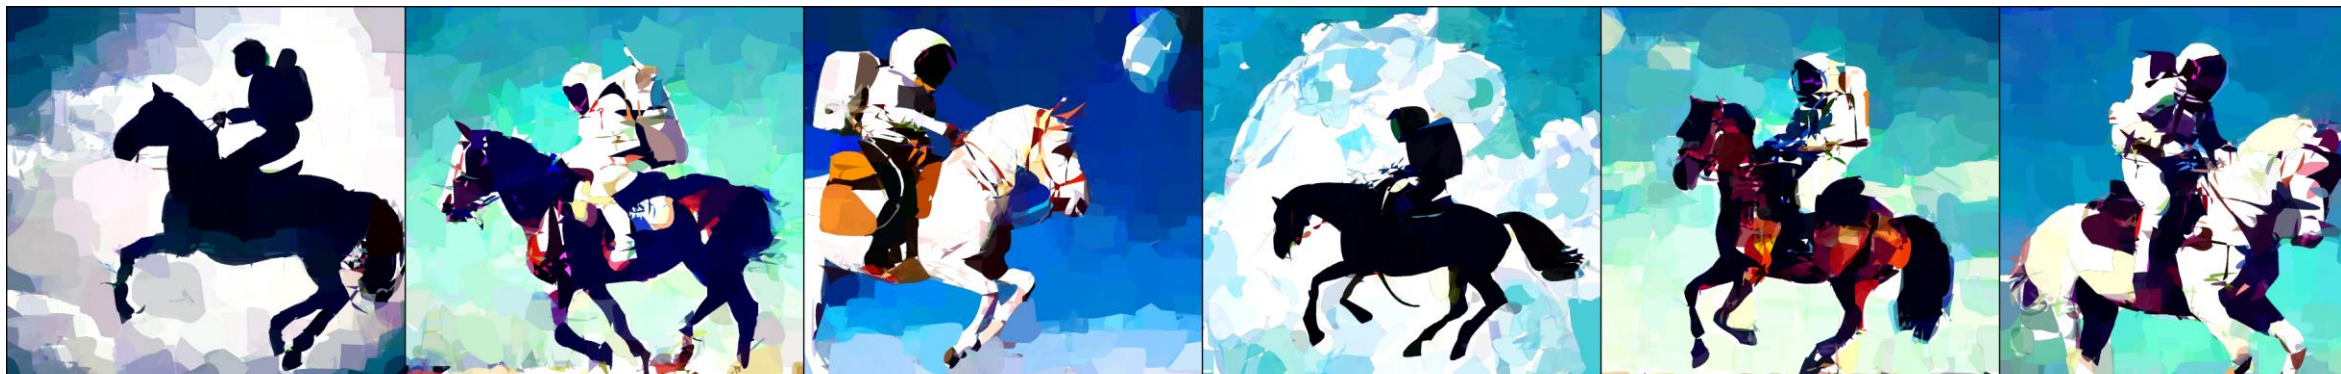



PSD  
=7.5

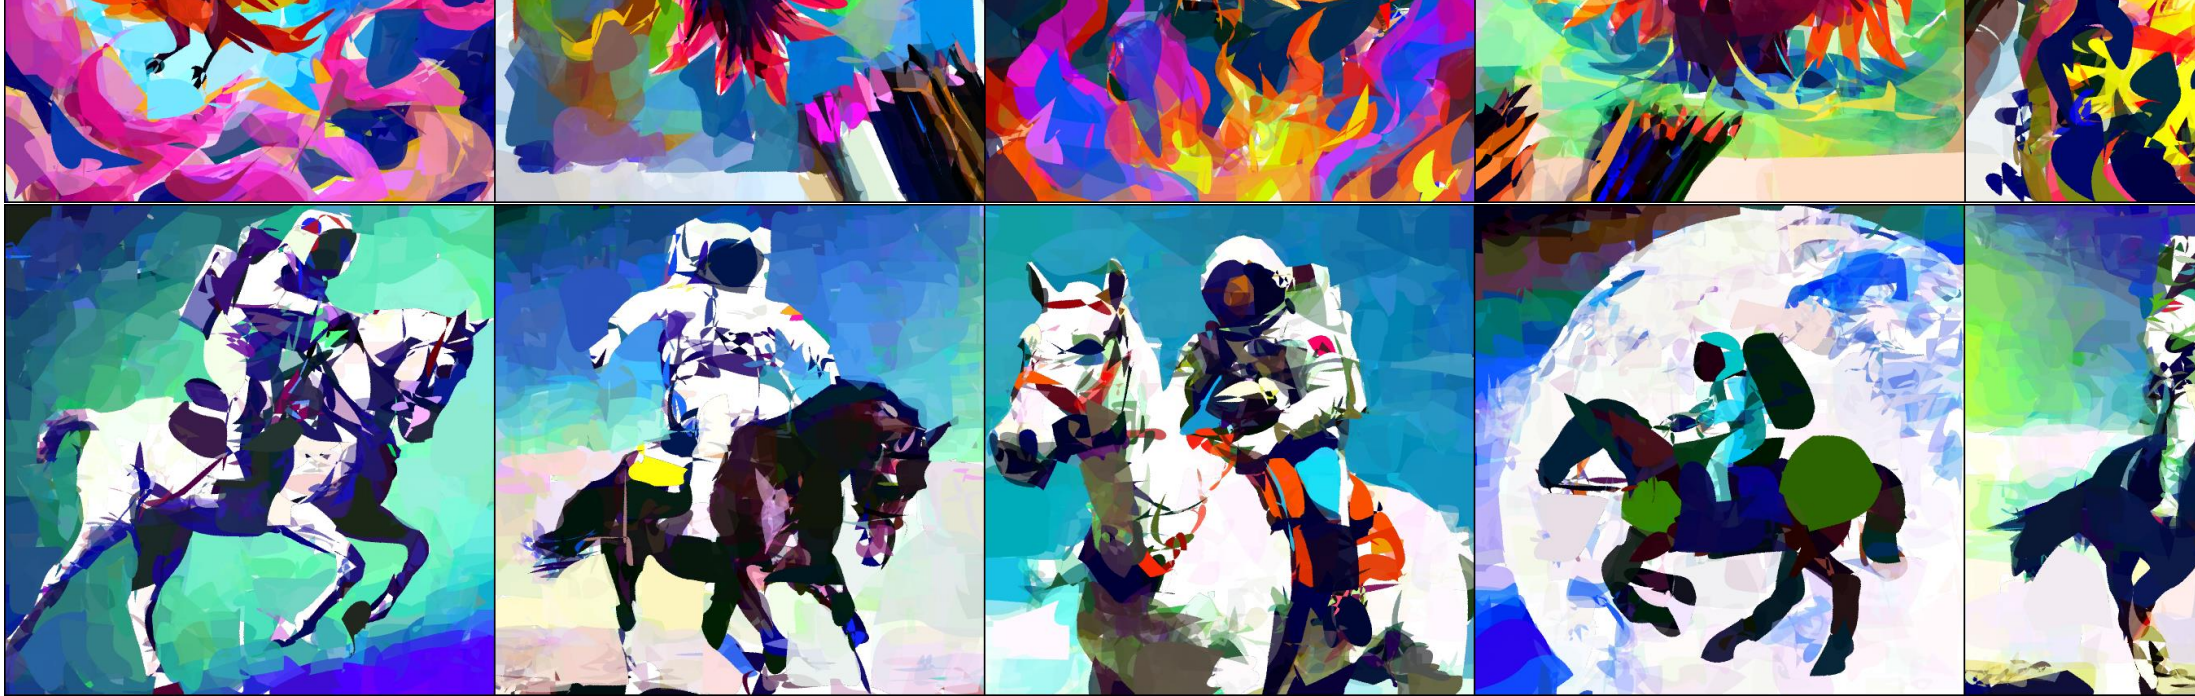

PSD  
G=2

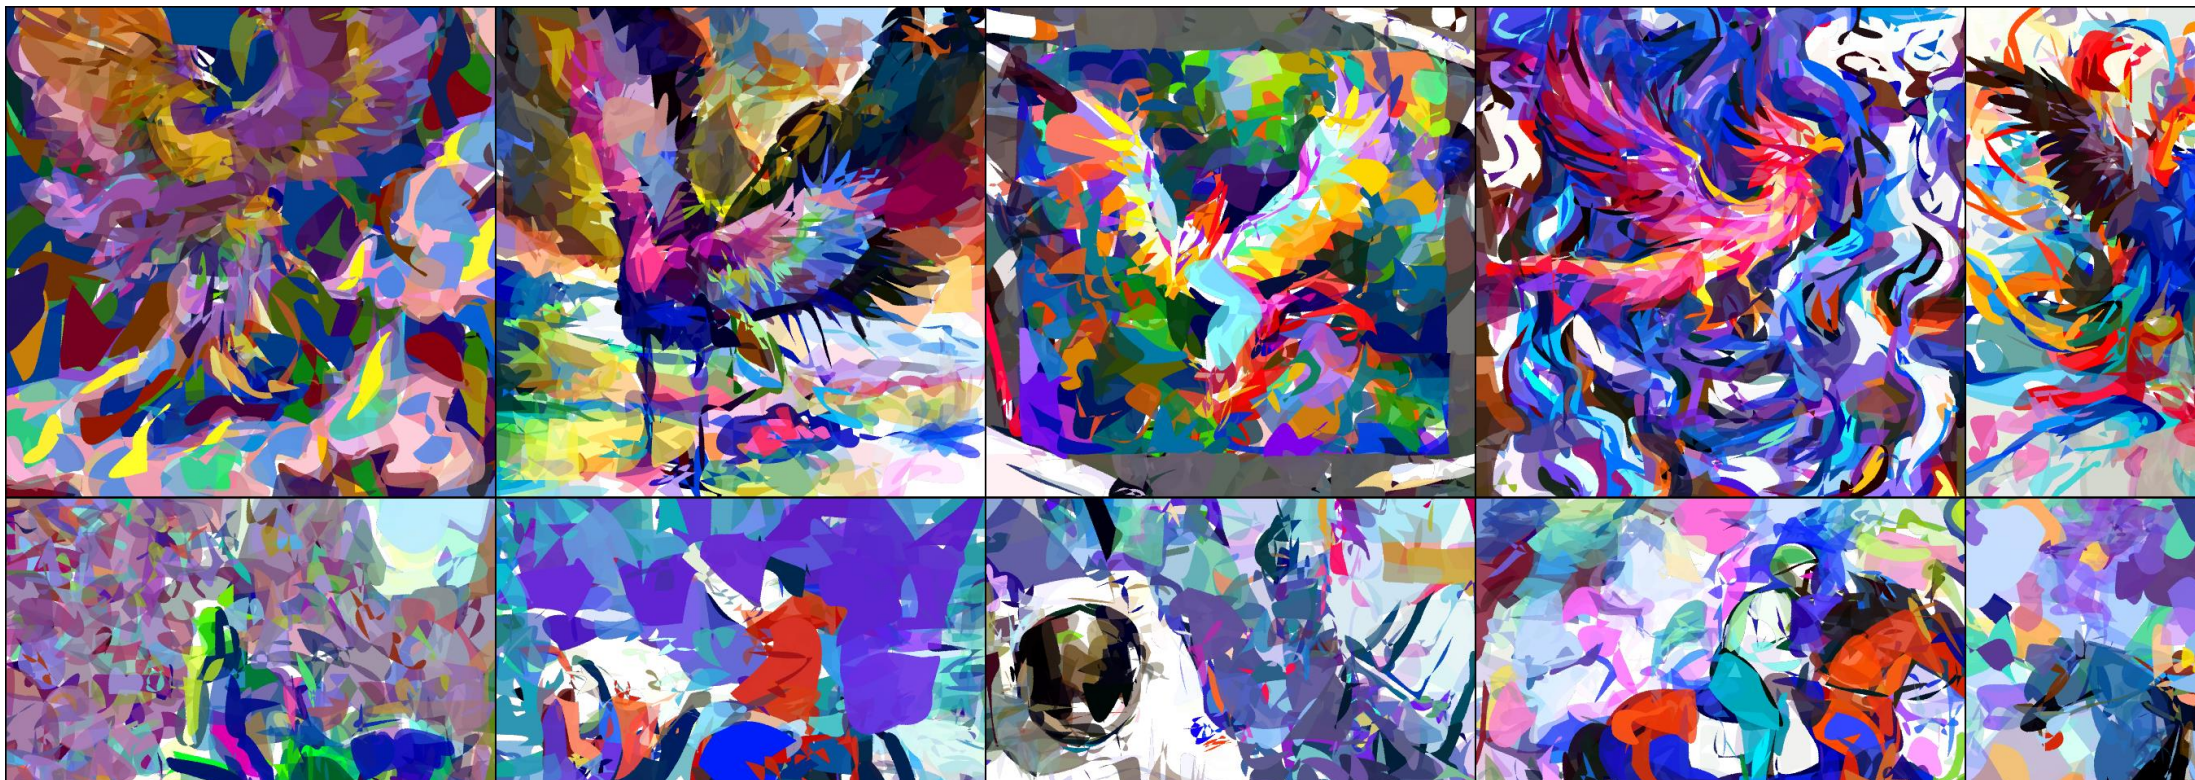



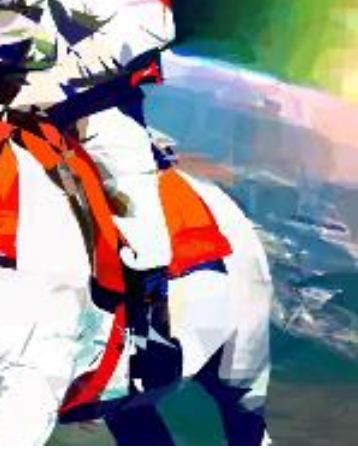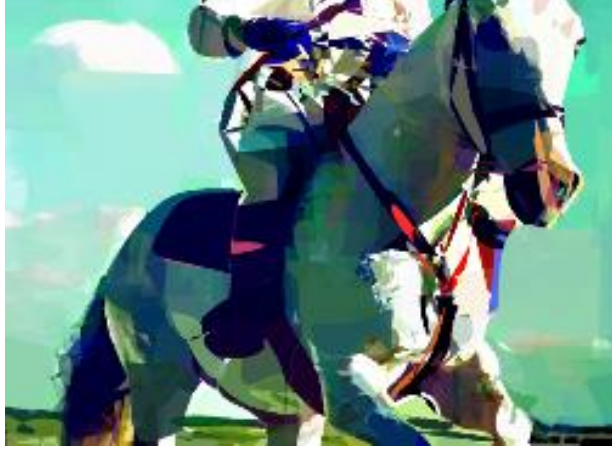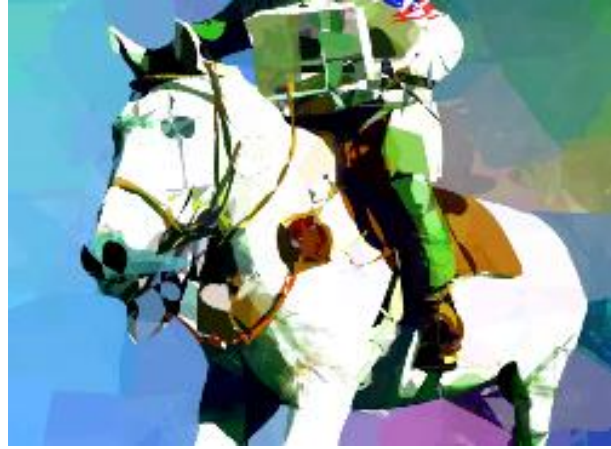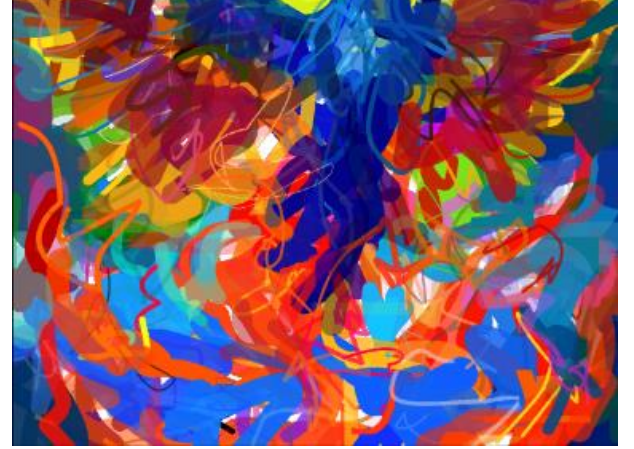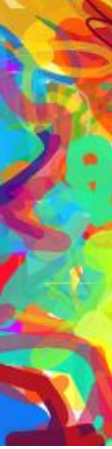

A photograph of an astronaut riding a horse.”

“A phoenix coming out of the ashes.”
